# Supplementary material for: Image Inpainting with Learnable Feature Imputation
Source: arXiv:2011.01077 source file (2020-11-02)
Supplement: Supplementary file 1 [file appendix.tex]

\title{\paperTitle \vspace{1em} (Supplementary)} % Replace with your title
\author{\paperAuthor}
\institute{\paperInstitute}
\titlerunning{\runningTitle} 
\authorrunning{\runningAuthor} 
\maketitle
\setcounter{page}{1}

The following items are included in the supplementary material:
\begin{enumerate}
	\item \appendixref{sec:gradient_penalty_exp} includes experiments analysing the impact of $L^\infty$ vs $L^2$ norm for gradient penalties.
	\item
	\appendixref{sec:appendix_experimental_section} details model architecture, hyperparameters and extensive experimental details.
	\item
	\appendixref{sec:appendix_quantitative} include additional quantitative results referenced to in the paper.
	\item
	\appendixref{sec:negative_results} shortly discuss negative results.
	\item
	\appendixref{sec:qualitative_other_papers_selections} includes a range of qualitative examples selected by previous authors.
	\item
	\appendixref{sec:appendix_deterministic_result} includes randomly sampled results on the FDF dataset, and examples illustrating our generator's ability of pluralistic image completion.
\end{enumerate}

\section{Alternative Gradient Penalty Norms}
\label{sec:gradient_penalty_exp}
\autoref{tab:gradient_penalty_comparison} shows Config A-E with $L^2$ gradient penalty replaced with $L^\infty$.
We find $L^\infty$ to get comparable quantitative resuls for most cnfigurations, except Config B where we significantly improve both FID and LPIPS.
%We find $L^\infty$ to improve our quantitative results for Config B; however, for all other configurations we observe similar .
We find a model trained with $L^\infty$ more sensitive to the choice of hyperparameters and we are not able to properly converge some configurations.
We theorize that this is due to $L^\infty$ nature of focusing on outliers.
% Can be moved to appendix
For each experiment, we keep the hyperparameters from the configurations in \autoref{tab:configurations}, replace the $L^2 \;$ norm with $L^\infty$, and we set $\lambda = 100$.

\begin{table}[t]
	
\caption{
	\textbf{Quantitative results of the impact of different gradient penalties}
	Quantitative results on the FDF dataset \cite{hukkelaas2019DeepPrivacy}.
	We report FID and LPIPS after showing the discriminator 30M images for Config A-D.
	For Config E, we report after showing the discriminator 20M images.
	*The training collapsed before reaching 30M images.
}
\centering
\resizebox{\textwidth}{!}{
\begin{tabular}{l|cc|cc|cc|cc|cc|cc}
	\hline
	\multirow{2}{*}{Gradient Penalty} & \multicolumn{2}{|c|}{Config A} & \multicolumn{2}{|c|}{Config B} & \multicolumn{2}{|c|}{Config C} & \multicolumn{2}{|c|}{Config D} & \multicolumn{2}{|c|}{Config E} \\
	 & FID & LPIPS (\%) & FID & LPIPS (\%) & FID & LPIPS (\%) & FID & LPIPS (\%) & FID & LPIPS (\%) \\
	\hline
	$L^2$ & 4.38 & 9.66 & 2.81 & 7.96 & \textbf{1.53} & \textbf{7.25} & \textbf{1.43} & \textbf{7.15} & \textbf{1.61} & \textbf{8.07} \\
	
	$L^\infty$ & --* & --* & \textbf{1.90} & \textbf{7.67} & 1.61 & 7.28 & 1.56 & 7.23 & 1.67 & 8.08 \\
	\hline

\end{tabular}}
\label{tab:gradient_penalty_comparison}
\end{table}

\section{Model architecture and hyperparameters}
\label{sec:appendix_experimental_section}

\subsection{Model Details}

We use the same discriminator architecture as \cite{hukkelaas2019DeepPrivacy}.
For the generator, we replace every convolution with our proposed input-estimated convolution (see \autoref{eq:our_method}).
The fully-connected pose pre-processing network consists of two fully connected layers.
The generator use 128 and 256 units for the pose network, while the discriminator use 64 and 1024 units.
Every fully connected layer use equalized learning rate \cite{karras2018progressive}, and is followed up by Leaky ReLU ($\alpha =0.2$) \cite{leakyReLU}.
We use average pool for downsampling and nearest neighbour upsampling.
In the generator we use Pixel Normalization \cite{karras2018progressive}.
Each convolution use equalized learning rate \cite{karras2018progressive}.

\subsubsection{Hyperparameters and Training Details}
We build upon the official pytorch implementation of DeepPrivacy \cite{hukkelaas2019DeepPrivacy}.
This setup corresponds to Config A in \autoref{tab:configurations}.
We keep all hyperparameters the same as \cite{hukkelaas2019DeepPrivacy}, except the following:
To train the network we use Adam \cite{adam} with a learning rate of 0.001 and a batch size of 256, 256, 128, 96, and 32 for resolution 8, 16, 32, 64, and 128.
We start progressive growing at $8 \times 8$ resolution and train for $1.2$M images.
We train the network for $2.4$M images per resolution for the following resolutions, .
We use an exponential running average for the weights of the generator, as this is shown to improve final image quality \cite{yazici2018the}.
For WGAN-GP we use $\lambda=10$ for all experiments, unless stated otherwise.
We enforce gradient penalty every 16th iteration (known as lazy-regularization \cite{karras2019analyzing}).
In combination with WGAN-GP we include a penalty to keep the discriminator from drifting away from zero, identical to \cite{karras2018progressive}.
All training is done with mixed precision training \cite{micikevicius2017mixed}.

For Flickr Diverse Faces \cite{hukkelaas2019DeepPrivacy}, we use the standard train/validation split of 1.42M for train and 50,000 images for validation.
To calculate LPIPS and FID, we use the pre-trained network and official implementations for each metric \cite{mescheder2018training,zhang2018perceptual}.
For all metrics reported in this work, we set the latent variable $z$ in the generator to all 0̈́'s.
For samples generated by \cite{zheng2019pluralistic} we set the seed to 0 before each forward pass.

\subsubsection{Places2 and CelebA-HQ experimental details}
\label{sec:free_form_experimental_details}
For Places2 \cite{places2} we use the standard train/validation split and use all categories, and for training we find a random crop of size $256 \times 256$ for places2.
For validation we use center crop of size $256 \times 256$.
For CelebA-HQ, we randomly sample 3,000 images as the validation set.
For each dataset, we generate random masks, following the approach in Yu \etal \cite{GatedConvolutionYu}.
We use the same hyperparameters from Config E, except that we include two convolution layers in the encoder and decoder of the generator, extending the network to $256 \times 256$ resolution.
We double the number of filters in each convolution, giving us a total of $11.5$M parameters in the generator.
Note that no other model design choices or hyperparameter tuning is done on these datasets.
Places2 model is trained until the discriminator has seen 20M images, while we train the CelebA-HQ model till 12M images.

\section{Additional Quantitative results}
\begin{figure}[H]
    \centering
    \begin{subfigure}{0.45\textwidth}
    \includegraphics[width=\textwidth]{images/ICONV_comparison_small.png}
%    \caption{Pconv \cite{PconvLiu}}
    \end{subfigure}
    \hspace{.01\textwidth}
    \begin{subfigure}{0.45\textwidth}
    \includegraphics[width=\textwidth]{images/ICONV_comparison_walltime_small.png}
%    \caption{Gated Conv \cite{GatedConvolutionYu}}
    \end{subfigure}
    \caption{LPIPS \cite{zhang2018perceptual} improvement during training our model with and without IConv for Places 2.}
    \label{fig:training_graph}
\end{figure}

\label{sec:appendix_quantitative}
\begin{table}
\caption{
	Quantitative results on the FDF dataset \cite{hukkelaas2019DeepPrivacy}.
	We report standard metrics after showing the discriminator 20M images.
	* Did not converge.
	$\dagger$ Same as Config B.}
\centering
\resizebox{\textwidth}{!}{
\begin{tabular}{ll|cccccc|cccccc}
	\hline
	\multicolumn{2}{l|}{Configuration} & \multicolumn{6}{c|}{FDF \cite{hukkelaas2019DeepPrivacy}} & \multicolumn{6}{c}{Places2 \cite{places2}} \\ 
	\hline
 &  & LPIPS $\downarrow$ & PSNR $\uparrow$ & FID $\downarrow$ & L1 $\downarrow$ & L2 $\downarrow$ & SSIM $\uparrow$ & LPIPS $\downarrow$ & PSNR $\uparrow$ & FID $\downarrow$ & L1 $\downarrow$ & L2 $\downarrow$ & SSIM $\uparrow$ \\

	A &  Baseline \cite{hukkelaas2019DeepPrivacy} & 22.52 & 0.1036 & 6.16 & 0.03 & 0.08 & 0.756 & --* & --* & --* & --* & --* & --* \\
B &  + Improved Gradient penalty & 0.0757 & 23.92 & 1.83 & 0.03 & 0.07 & 0.787 & 0.1619 & 20.99 & 7.96 & 0.03 & 0.10 & 0.747 \\
C & + Scalar Pose Information & 0.0733 & 24.01 & 1.76 & 0.02 & 0.07 & 0.791 & --$\dagger$ & --$\dagger$ & --$\dagger$ & --$\dagger$ & --$\dagger$ & --$\dagger$ \\
D & + Learned Pool & 0.0739 & 23.95 & 1.66 & 0.03 & 0.07 & 0.790 & 0.1563 & 21.21 & 6.81 & 0.03 & 0.10 & 0.749 \\
\hline
E & + No Growing, MSG & 0.0728 & 24.01 & 1.49 & 0.02 & 0.07 & 0.790 & 0.1491 & 21.42 & 5.24 & 0.03 & 0.10 & 0.752 \\

\end{tabular}}
\label{tab:configurations_full}
\end{table}

\section{Negative Results and Minor Observations}
\label{sec:negative_results}
We explored several novel and existing techniques to improve GAN-based image inpainting.
For several techniques, we found a negative impact on generated image quality, or we did not see significant improvement.
We report these results to guide further work and help save time.
We note that these results are not as thorough as those presented in the paper, and each result is observed on the FDF dataset ($128 \times 128 \;$ resolution).
\begin{itemize}
	\item Following the number of parameter analysis of \cite{karras2019analyzing}, we observe that approximately $40\%$ of the generated image is from the $256 \times 256$ toRGB module on the CelebA-HQ and Places2 datasets.
	This indicates that the network might benefit of an increase in number of parameters; however, due to computational limitation we were not able to test this further.
	 
	\item We tried adding dilation to $h_x$ and saw no significant difference. 
	However, we did not change the dilation rate depending on the resolution, which could be beneficial.
	\item We tried adding dilated convolution in the generator and discriminator for the resolution 128, 64 and 32.
	However, we observed no major benefit.
	\item We tried to remove the conditional pose information  to the discriminator and instead let the discriminator predict it, motivated by auxiliary-classifier GAN in \cite{odena2017conditional}.
	This significantly degraded final LPIPS score on the FDF dataset.
	
\end{itemize}

\section{More Qualitative results}
\label{sec:qualitative_other_papers_selections}
We present qualitative results on images presented in recent image-inpainting models \cite{Guo_2019,BidirectionalAttentionXie,GatedConvolutionYu,zheng2019pluralistic}.
\begin{enumerate}
	\item 
	Examples selected by Zheng \etal \cite{zheng2019pluralistic} can be seen in  \autoref{fig:pluralistic_0}, and \autoref{fig:pluralistic_1}.
	\item
	Examples selected by Yu \etal \cite{GatedConvolutionYu} can be seen in 
	\autoref{fig:gated_conv_places2_0}, and \autoref{fig:gated_conv_places2_1}.  
	\item
	Examples selected by Xie \etal \cite{BidirectionalAttentionXie} can be seen in \autoref{fig:LBAM_0}, \autoref{fig:LBAM_1}, \autoref{fig:LBAM_2}, \autoref{fig:LBAM_3}, and \autoref{fig:LBAM_4}.
	\autoref{fig:LBAM_0} represents difficult failure cases for \cite{BidirectionalAttentionXie}.
	\item Examples selected by Guo \etal \cite{Guo_2019} can be seen in \autoref{fig:FRRN_0}
\end{enumerate}

\subsection{Randomly Sampled}
\label{sec:random_sample_qualitative}
We randomly sample examples of the CelebA-HQ and Places2 validation datasets, shown in \autoref{tab:dataset_comparisons}.
\begin{enumerate}
	\item For CelebA-HQ center crop, see \autoref{fig:celebA-HQ_randomly_0} and  \autoref{fig:celebA-HQ_randomly_1}.
	
	\item For CelebA-HQ free-form, see \autoref{fig:celebA-HQ_free_form_randomly_0} and \autoref{fig:celebA-HQ_free_form_randomly_1}.
	
	\item For Places2 center crop, see \autoref{fig:places2_randomly_0} and \autoref{fig:places2_randomly_1}.
	
	\item For Places2 free-form, see \autoref{fig:places2_free_form_randomly_0} and \autoref{fig:places2_free_form_randomly_1}.
\end{enumerate}

\subsubsection{Selection Methodology}
We select qualitative examples picked by previous authors whom address  the issue of free-form image inpainting \cite{Guo_2019,GatedConvolutionYu,BidirectionalAttentionXie}, or presents high quality inpainted examples with free-form masks \cite{zheng2019pluralistic}.
From these papers, we select all qualitative examples that are present in their original camera ready paper, supplementary material, or in the official source code.
Given the images included from these sources, we select all:
\begin{enumerate}
	\item Images stored without compression (.png files), where we are able to retrieve both the mask and the original image (or masked out image).
	\item A few examples stored with compression, from \cite{zheng2019pluralistic}.
	Retrieving the original binary mask from a masked out image and the original images is extremely time consuming, and we decided to only select samples from the CelebA-HQ dataset with free-form masks.
\end{enumerate}
We will publish all of these qualitative examples uncompressed in an easy to download format, to save time for further work.

\section{Deterministic Experiment}
\label{sec:appendix_deterministic_result}
We select 10 samples to show diverse samplings from our generator in \autoref{fig:deterministc_experiment_appendix}.
Furthermore, we select 10 samples \textit{randomly} in \autoref{fig:deterministc_experiment_appendix_random}.

\newpage
\begin{figure}[t]
\centering
\begin{subfigure}[t]{0.25\textwidth}
\includegraphics[width=\textwidth]{images/comparisons/pluralistic/celebA_HQ/masked_out/1.png}
\includegraphics[width=\textwidth]{images/comparisons/pluralistic/celebA_HQ/masked_out/2.png}
\includegraphics[width=\textwidth]{images/comparisons/pluralistic/celebA_HQ/masked_out/3.png}
\caption{Input}
\end{subfigure}%%
\begin{subfigure}[t]{0.25\textwidth}
\includegraphics[width=\textwidth]{images/comparisons/pluralistic/celebA_HQ/gated_conv/1.png}
\includegraphics[width=\textwidth]{images/comparisons/pluralistic/celebA_HQ/gated_conv/2.png}
\includegraphics[width=\textwidth]{images/comparisons/pluralistic/celebA_HQ/gated_conv/3.png}
\caption{GConv \cite{GatedConvolutionYu}}
\end{subfigure}%%
\begin{subfigure}[t]{0.25\textwidth}
\includegraphics[width=\textwidth]{images/comparisons/pluralistic/celebA_HQ/pluralistic/1.png}
\includegraphics[width=\textwidth]{images/comparisons/pluralistic/celebA_HQ/pluralistic/2.png}
\includegraphics[width=\textwidth]{images/comparisons/pluralistic/celebA_HQ/pluralistic/3.png}
\caption{PIC \cite{zheng2019pluralistic}}
\end{subfigure}%%
\begin{subfigure}[t]{0.25\textwidth}
\includegraphics[width=\textwidth]{images/comparisons/pluralistic/celebA_HQ/result/1.png}
\includegraphics[width=\textwidth]{images/comparisons/pluralistic/celebA_HQ/result/2.png}
\includegraphics[width=\textwidth]{images/comparisons/pluralistic/celebA_HQ/result/3.png}
\caption{Ours}
\end{subfigure}%%
\caption{\textbf{CelebA-HQ comparison to state-of-the-art models}
Examples selected by authors of \cite{zheng2019pluralistic} (images extracted from their paper and supplementary material).
Due to the original images and masks being stored in .jpg format with compression, the results might differ from original paper.
Therefore, we decided to generate results from \cite{zheng2019pluralistic} again.
Results of \cite{GatedConvolutionYu,zheng2019pluralistic} generated by using their open-source code and models.
Note that the original image size is $256 \times 256$.
We recommend the reader to zoom-in on missing regions.}
\label{fig:pluralistic_0}
\end{figure}
\begin{figure}[t]
\centering
\begin{subfigure}[t]{0.25\textwidth}
\includegraphics[width=\textwidth]{images/comparisons/pluralistic/celebA_HQ/masked_out/4.png}
\includegraphics[width=\textwidth]{images/comparisons/pluralistic/celebA_HQ/masked_out/5.png}
\includegraphics[width=\textwidth]{images/comparisons/pluralistic/celebA_HQ/masked_out/6.png}
\caption{Input}
\end{subfigure}%%
\begin{subfigure}[t]{0.25\textwidth}
\includegraphics[width=\textwidth]{images/comparisons/pluralistic/celebA_HQ/gated_conv/4.png}
\includegraphics[width=\textwidth]{images/comparisons/pluralistic/celebA_HQ/gated_conv/5.png}
\includegraphics[width=\textwidth]{images/comparisons/pluralistic/celebA_HQ/gated_conv/6.png}
\caption{GConv \cite{GatedConvolutionYu}}
\end{subfigure}%%
\begin{subfigure}[t]{0.25\textwidth}
\includegraphics[width=\textwidth]{images/comparisons/pluralistic/celebA_HQ/pluralistic/4.png}
\includegraphics[width=\textwidth]{images/comparisons/pluralistic/celebA_HQ/pluralistic/5.png}
\includegraphics[width=\textwidth]{images/comparisons/pluralistic/celebA_HQ/pluralistic/6.png}
\caption{PIC \cite{zheng2019pluralistic}}
\end{subfigure}%%
\begin{subfigure}[t]{0.25\textwidth}
\includegraphics[width=\textwidth]{images/comparisons/pluralistic/celebA_HQ/result/4.png}
\includegraphics[width=\textwidth]{images/comparisons/pluralistic/celebA_HQ/result/5.png}
\includegraphics[width=\textwidth]{images/comparisons/pluralistic/celebA_HQ/result/6.png}
\caption{Ours}
\end{subfigure}%%
\caption{\textbf{CelebA-HQ comparison to state-of-the-art models}
Examples selected by authors of \cite{zheng2019pluralistic} (images extracted from their paper and supplementary material).
Due to the original images and masks being stored in .jpg format with compression, the results might differ from original paper.
Therefore, we decided to generate results from \cite{zheng2019pluralistic} again.
Results of \cite{GatedConvolutionYu,zheng2019pluralistic} generated by using their open-source code and models.
Note that the original image size is $256 \times 256$.
We recommend the reader to zoom-in on missing regions.}
\label{fig:pluralistic_1}
\end{figure}

\begin{figure}[t]
\centering
\begin{subfigure}[t]{0.25\textwidth}
\includegraphics[width=\textwidth]{images/comparisons/gated_conv/places2/masked_out/1.png}
\includegraphics[width=\textwidth]{images/comparisons/gated_conv/places2/masked_out/2.png}
\includegraphics[width=\textwidth]{images/comparisons/gated_conv/places2/masked_out/3.png}
\caption{Input}
\end{subfigure}%%
\begin{subfigure}[t]{0.25\textwidth}
\includegraphics[width=\textwidth]{images/comparisons/gated_conv/places2/gated_conv/1.png}
\includegraphics[width=\textwidth]{images/comparisons/gated_conv/places2/gated_conv/2.png}
\includegraphics[width=\textwidth]{images/comparisons/gated_conv/places2/gated_conv/3.png}
\caption{GConv \cite{GatedConvolutionYu}}
\end{subfigure}%%
\begin{subfigure}[t]{0.25\textwidth}
\includegraphics[width=\textwidth]{images/comparisons/gated_conv/places2/pluralistic/1.png}
\includegraphics[width=\textwidth]{images/comparisons/gated_conv/places2/pluralistic/2.png}
\includegraphics[width=\textwidth]{images/comparisons/gated_conv/places2/pluralistic/3.png}
\caption{PIC \cite{zheng2019pluralistic}}
\end{subfigure}%%
\begin{subfigure}[t]{0.25\textwidth}
\includegraphics[width=\textwidth]{images/comparisons/gated_conv/places2/result/1.png}
\includegraphics[width=\textwidth]{images/comparisons/gated_conv/places2/result/2.png}
\includegraphics[width=\textwidth]{images/comparisons/gated_conv/places2/result/3.png}
\caption{Ours}
\end{subfigure}%%
\caption{\textbf{Places2 comparison to state-of-the-art models}
Examples selected by authors of \cite{GatedConvolutionYu} (images extracted from their official github page).
Results of \cite{zheng2019pluralistic} generated by using their open-source code and models.
Note that original image size is $512 \times 680$.
Our network and \cite{zheng2019pluralistic} expects image size of $256 \times 256$, therefore we resize the input image.
We recommend the reader to zoom-in on missing regions.}
\label{fig:gated_conv_places2_0}
\end{figure}
\begin{figure}[t]
\centering
\begin{subfigure}[t]{0.25\textwidth}
\includegraphics[width=\textwidth]{images/comparisons/gated_conv/places2/masked_out/4.png}
\includegraphics[width=\textwidth]{images/comparisons/gated_conv/places2/masked_out/5.png}
\includegraphics[width=\textwidth]{images/comparisons/gated_conv/places2/masked_out/6.png}
\caption{Input}
\end{subfigure}%%
\begin{subfigure}[t]{0.25\textwidth}
\includegraphics[width=\textwidth]{images/comparisons/gated_conv/places2/gated_conv/4.png}
\includegraphics[width=\textwidth]{images/comparisons/gated_conv/places2/gated_conv/5.png}
\includegraphics[width=\textwidth]{images/comparisons/gated_conv/places2/gated_conv/6.png}
\caption{GConv \cite{GatedConvolutionYu}}
\end{subfigure}%%
\begin{subfigure}[t]{0.25\textwidth}
\includegraphics[width=\textwidth]{images/comparisons/gated_conv/places2/pluralistic/4.png}
\includegraphics[width=\textwidth]{images/comparisons/gated_conv/places2/pluralistic/5.png}
\includegraphics[width=\textwidth]{images/comparisons/gated_conv/places2/pluralistic/6.png}
\caption{PIC \cite{zheng2019pluralistic}}
\end{subfigure}%%
\begin{subfigure}[t]{0.25\textwidth}
\includegraphics[width=\textwidth]{images/comparisons/gated_conv/places2/result/4.png}
\includegraphics[width=\textwidth]{images/comparisons/gated_conv/places2/result/5.png}
\includegraphics[width=\textwidth]{images/comparisons/gated_conv/places2/result/6.png}
\caption{Ours}
\end{subfigure}%%
\caption{\textbf{Places2 comparison to state-of-the-art models}
Examples selected by authors of \cite{GatedConvolutionYu} (images extracted from their official github page).
Results of \cite{zheng2019pluralistic} generated by using their open-source code and models.
Note that original image size is $512 \times 680$.
Our network and \cite{zheng2019pluralistic} expects image size of $256 \times 256$, therefore we resize the input image.
We recommend the reader to zoom-in on missing regions.}
\label{fig:gated_conv_places2_1}
\end{figure}
\begin{figure}[t]
\centering
\begin{subfigure}[t]{0.2\textwidth}
\includegraphics[width=\textwidth]{images/comparisons/LBAM/places2/masked_out/1.png}
\includegraphics[width=\textwidth]{images/comparisons/LBAM/places2/masked_out/2.png}
\includegraphics[width=\textwidth]{images/comparisons/LBAM/places2/masked_out/3.png}
\includegraphics[width=\textwidth]{images/comparisons/LBAM/places2/masked_out/4.png}
\includegraphics[width=\textwidth]{images/comparisons/LBAM/places2/masked_out/5.png}
\includegraphics[width=\textwidth]{images/comparisons/LBAM/places2/masked_out/6.png}
\caption{Input}
\end{subfigure}%%
\begin{subfigure}[t]{0.2\textwidth}
\includegraphics[width=\textwidth]{images/comparisons/LBAM/places2/LBAM/1.png}
\includegraphics[width=\textwidth]{images/comparisons/LBAM/places2/LBAM/2.png}
\includegraphics[width=\textwidth]{images/comparisons/LBAM/places2/LBAM/3.png}
\includegraphics[width=\textwidth]{images/comparisons/LBAM/places2/LBAM/4.png}
\includegraphics[width=\textwidth]{images/comparisons/LBAM/places2/LBAM/5.png}
\includegraphics[width=\textwidth]{images/comparisons/LBAM/places2/LBAM/6.png}
\caption{LBAM \cite{BidirectionalAttentionXie}}
\end{subfigure}%%
\begin{subfigure}[t]{0.2\textwidth}
\includegraphics[width=\textwidth]{images/comparisons/LBAM/places2/gated_conv/1.png}
\includegraphics[width=\textwidth]{images/comparisons/LBAM/places2/gated_conv/2.png}
\includegraphics[width=\textwidth]{images/comparisons/LBAM/places2/gated_conv/3.png}
\includegraphics[width=\textwidth]{images/comparisons/LBAM/places2/gated_conv/4.png}
\includegraphics[width=\textwidth]{images/comparisons/LBAM/places2/gated_conv/5.png}
\includegraphics[width=\textwidth]{images/comparisons/LBAM/places2/gated_conv/6.png}
\caption{GConv \cite{GatedConvolutionYu}}
\end{subfigure}%%
\begin{subfigure}[t]{0.2\textwidth}
\includegraphics[width=\textwidth]{images/comparisons/LBAM/places2/pluralistic/1.png}
\includegraphics[width=\textwidth]{images/comparisons/LBAM/places2/pluralistic/2.png}
\includegraphics[width=\textwidth]{images/comparisons/LBAM/places2/pluralistic/3.png}
\includegraphics[width=\textwidth]{images/comparisons/LBAM/places2/pluralistic/4.png}
\includegraphics[width=\textwidth]{images/comparisons/LBAM/places2/pluralistic/5.png}
\includegraphics[width=\textwidth]{images/comparisons/LBAM/places2/pluralistic/6.png}
\caption{PIC \cite{zheng2019pluralistic}}
\end{subfigure}%%
\begin{subfigure}[t]{0.2\textwidth}
\includegraphics[width=\textwidth]{images/comparisons/LBAM/places2/result/1.png}
\includegraphics[width=\textwidth]{images/comparisons/LBAM/places2/result/2.png}
\includegraphics[width=\textwidth]{images/comparisons/LBAM/places2/result/3.png}
\includegraphics[width=\textwidth]{images/comparisons/LBAM/places2/result/4.png}
\includegraphics[width=\textwidth]{images/comparisons/LBAM/places2/result/5.png}
\includegraphics[width=\textwidth]{images/comparisons/LBAM/places2/result/6.png}
\caption{Ours}
\end{subfigure}%%
\caption{\textbf{Places2 comparison to state-of-the-art models}
Examples selected by authors of \cite{BidirectionalAttentionXie} (images extracted from their supplementary material).
Results of \cite{GatedConvolutionYu,zheng2019pluralistic} generated by using their open-source code and models.
For comparisons to Patchmatch \cite{Barnes_2009}, Global \& Local Attention \cite{Iizuka_2017}, Contextual Attention \cite{ConextualAttention2018Yu}  and Partial Conv \cite{PconvLiu}, see \cite{BidirectionalAttentionXie}.
We recommend the reader to zoom-in on missing regions.
The top two rows is presented as \textbf{failure cases} by the authors of \cite{BidirectionalAttentionXie}.}
\label{fig:LBAM_0}
\end{figure}
\begin{figure}[t]
\centering
\begin{subfigure}[t]{0.2\textwidth}
\includegraphics[width=\textwidth]{images/comparisons/LBAM/places2/masked_out/7.png}
\includegraphics[width=\textwidth]{images/comparisons/LBAM/places2/masked_out/8.png}
\includegraphics[width=\textwidth]{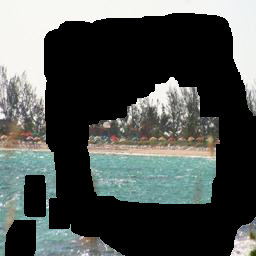}
\includegraphics[width=\textwidth]{images/comparisons/LBAM/places2/masked_out/10.png}
\includegraphics[width=\textwidth]{images/comparisons/LBAM/places2/masked_out/11.png}
\includegraphics[width=\textwidth]{images/comparisons/LBAM/places2/masked_out/12.png}
\caption{Input}
\end{subfigure}%%
\begin{subfigure}[t]{0.2\textwidth}
\includegraphics[width=\textwidth]{images/comparisons/LBAM/places2/LBAM/7.png}
\includegraphics[width=\textwidth]{images/comparisons/LBAM/places2/LBAM/8.png}
\includegraphics[width=\textwidth]{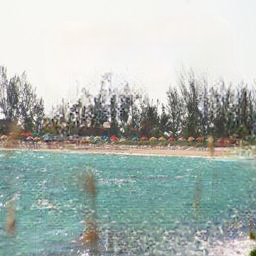}
\includegraphics[width=\textwidth]{images/comparisons/LBAM/places2/LBAM/10.png}
\includegraphics[width=\textwidth]{images/comparisons/LBAM/places2/LBAM/11.png}
\includegraphics[width=\textwidth]{images/comparisons/LBAM/places2/LBAM/12.png}
\caption{LBAM \cite{BidirectionalAttentionXie}}
\end{subfigure}%%
\begin{subfigure}[t]{0.2\textwidth}
\includegraphics[width=\textwidth]{images/comparisons/LBAM/places2/gated_conv/7.png}
\includegraphics[width=\textwidth]{images/comparisons/LBAM/places2/gated_conv/8.png}
\includegraphics[width=\textwidth]{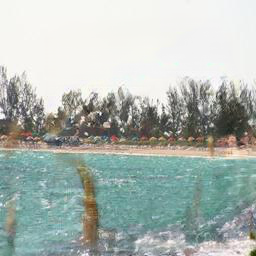}
\includegraphics[width=\textwidth]{images/comparisons/LBAM/places2/gated_conv/10.png}
\includegraphics[width=\textwidth]{images/comparisons/LBAM/places2/gated_conv/11.png}
\includegraphics[width=\textwidth]{images/comparisons/LBAM/places2/gated_conv/12.png}
\caption{GConv \cite{GatedConvolutionYu}}
\end{subfigure}%%
\begin{subfigure}[t]{0.2\textwidth}
\includegraphics[width=\textwidth]{images/comparisons/LBAM/places2/pluralistic/7.png}
\includegraphics[width=\textwidth]{images/comparisons/LBAM/places2/pluralistic/8.png}
\includegraphics[width=\textwidth]{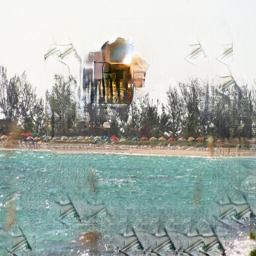}
\includegraphics[width=\textwidth]{images/comparisons/LBAM/places2/pluralistic/10.png}
\includegraphics[width=\textwidth]{images/comparisons/LBAM/places2/pluralistic/11.png}
\includegraphics[width=\textwidth]{images/comparisons/LBAM/places2/pluralistic/12.png}
\caption{PIC \cite{zheng2019pluralistic}}
\end{subfigure}%%
\begin{subfigure}[t]{0.2\textwidth}
\includegraphics[width=\textwidth]{images/comparisons/LBAM/places2/result/7.png}
\includegraphics[width=\textwidth]{images/comparisons/LBAM/places2/result/8.png}
\includegraphics[width=\textwidth]{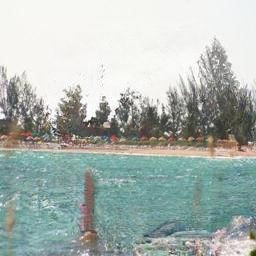}
\includegraphics[width=\textwidth]{images/comparisons/LBAM/places2/result/10.png}
\includegraphics[width=\textwidth]{images/comparisons/LBAM/places2/result/11.png}
\includegraphics[width=\textwidth]{images/comparisons/LBAM/places2/result/12.png}
\caption{Ours}
\end{subfigure}%%
\caption{\textbf{Places2 comparison to state-of-the-art models}
Examples selected by authors of \cite{BidirectionalAttentionXie} (images extracted from their supplementary material).
Results of \cite{GatedConvolutionYu,zheng2019pluralistic} generated by using their open-source code and models.
For comparisons to Patchmatch \cite{Barnes_2009}, Global \& Local Attention \cite{Iizuka_2017}, Contextual Attention \cite{ConextualAttention2018Yu}  and Partial Conv \cite{PconvLiu}, see \cite{BidirectionalAttentionXie}.
We recommend the reader to zoom-in on missing regions.}
\label{fig:LBAM_1}
\end{figure}
\begin{figure}[t]
\centering
\begin{subfigure}[t]{0.2\textwidth}
\includegraphics[width=\textwidth]{images/comparisons/LBAM/places2/masked_out/13.png}
\includegraphics[width=\textwidth]{images/comparisons/LBAM/places2/masked_out/14.png}
\includegraphics[width=\textwidth]{images/comparisons/LBAM/places2/masked_out/15.png}
\includegraphics[width=\textwidth]{images/comparisons/LBAM/places2/masked_out/16.png}
\includegraphics[width=\textwidth]{images/comparisons/LBAM/places2/masked_out/17.png}
\includegraphics[width=\textwidth]{images/comparisons/LBAM/places2/masked_out/18.png}
\caption{Input}
\end{subfigure}%%
\begin{subfigure}[t]{0.2\textwidth}
\includegraphics[width=\textwidth]{images/comparisons/LBAM/places2/LBAM/13.png}
\includegraphics[width=\textwidth]{images/comparisons/LBAM/places2/LBAM/14.png}
\includegraphics[width=\textwidth]{images/comparisons/LBAM/places2/LBAM/15.png}
\includegraphics[width=\textwidth]{images/comparisons/LBAM/places2/LBAM/16.png}
\includegraphics[width=\textwidth]{images/comparisons/LBAM/places2/LBAM/17.png}
\includegraphics[width=\textwidth]{images/comparisons/LBAM/places2/LBAM/18.png}
\caption{LBAM \cite{BidirectionalAttentionXie}}
\end{subfigure}%%
\begin{subfigure}[t]{0.2\textwidth}
\includegraphics[width=\textwidth]{images/comparisons/LBAM/places2/gated_conv/13.png}
\includegraphics[width=\textwidth]{images/comparisons/LBAM/places2/gated_conv/14.png}
\includegraphics[width=\textwidth]{images/comparisons/LBAM/places2/gated_conv/15.png}
\includegraphics[width=\textwidth]{images/comparisons/LBAM/places2/gated_conv/16.png}
\includegraphics[width=\textwidth]{images/comparisons/LBAM/places2/gated_conv/17.png}
\includegraphics[width=\textwidth]{images/comparisons/LBAM/places2/gated_conv/18.png}
\caption{GConv \cite{GatedConvolutionYu}}
\end{subfigure}%%
\begin{subfigure}[t]{0.2\textwidth}
\includegraphics[width=\textwidth]{images/comparisons/LBAM/places2/pluralistic/13.png}
\includegraphics[width=\textwidth]{images/comparisons/LBAM/places2/pluralistic/14.png}
\includegraphics[width=\textwidth]{images/comparisons/LBAM/places2/pluralistic/15.png}
\includegraphics[width=\textwidth]{images/comparisons/LBAM/places2/pluralistic/16.png}
\includegraphics[width=\textwidth]{images/comparisons/LBAM/places2/pluralistic/17.png}
\includegraphics[width=\textwidth]{images/comparisons/LBAM/places2/pluralistic/18.png}
\caption{PIC \cite{zheng2019pluralistic}}
\end{subfigure}%%
\begin{subfigure}[t]{0.2\textwidth}
\includegraphics[width=\textwidth]{images/comparisons/LBAM/places2/result/13.png}
\includegraphics[width=\textwidth]{images/comparisons/LBAM/places2/result/14.png}
\includegraphics[width=\textwidth]{images/comparisons/LBAM/places2/result/15.png}
\includegraphics[width=\textwidth]{images/comparisons/LBAM/places2/result/16.png}
\includegraphics[width=\textwidth]{images/comparisons/LBAM/places2/result/17.png}
\includegraphics[width=\textwidth]{images/comparisons/LBAM/places2/result/18.png}
\caption{Ours}
\end{subfigure}%%
\caption{\textbf{Places2 comparison to state-of-the-art models}
Examples selected by authors of \cite{BidirectionalAttentionXie} (images extracted from their supplementary material).
Results of \cite{GatedConvolutionYu,zheng2019pluralistic} generated by using their open-source code and models.
For comparisons to Patchmatch \cite{Barnes_2009}, Global \& Local Attention \cite{Iizuka_2017}, Contextual Attention \cite{ConextualAttention2018Yu}  and Partial Conv \cite{PconvLiu}, see \cite{BidirectionalAttentionXie}.
We recommend the reader to zoom-in on missing regions.}
\label{fig:LBAM_2}
\end{figure}
\begin{figure}[t]
\centering
\begin{subfigure}[t]{0.2\textwidth}
\includegraphics[width=\textwidth]{images/comparisons/LBAM/places2/masked_out/19.png}
\includegraphics[width=\textwidth]{images/comparisons/LBAM/places2/masked_out/20.png}
\includegraphics[width=\textwidth]{images/comparisons/LBAM/places2/masked_out/21.png}
\includegraphics[width=\textwidth]{images/comparisons/LBAM/places2/masked_out/22.png}
\includegraphics[width=\textwidth]{images/comparisons/LBAM/places2/masked_out/23.png}
\includegraphics[width=\textwidth]{images/comparisons/LBAM/places2/masked_out/24.png}
\caption{Input}
\end{subfigure}%%
\begin{subfigure}[t]{0.2\textwidth}
\includegraphics[width=\textwidth]{images/comparisons/LBAM/places2/LBAM/19.png}
\includegraphics[width=\textwidth]{images/comparisons/LBAM/places2/LBAM/20.png}
\includegraphics[width=\textwidth]{images/comparisons/LBAM/places2/LBAM/21.png}
\includegraphics[width=\textwidth]{images/comparisons/LBAM/places2/LBAM/22.png}
\includegraphics[width=\textwidth]{images/comparisons/LBAM/places2/LBAM/23.png}
\includegraphics[width=\textwidth]{images/comparisons/LBAM/places2/LBAM/24.png}
\caption{LBAM \cite{BidirectionalAttentionXie}}
\end{subfigure}%%
\begin{subfigure}[t]{0.2\textwidth}
\includegraphics[width=\textwidth]{images/comparisons/LBAM/places2/gated_conv/19.png}
\includegraphics[width=\textwidth]{images/comparisons/LBAM/places2/gated_conv/20.png}
\includegraphics[width=\textwidth]{images/comparisons/LBAM/places2/gated_conv/21.png}
\includegraphics[width=\textwidth]{images/comparisons/LBAM/places2/gated_conv/22.png}
\includegraphics[width=\textwidth]{images/comparisons/LBAM/places2/gated_conv/23.png}
\includegraphics[width=\textwidth]{images/comparisons/LBAM/places2/gated_conv/24.png}
\caption{GConv \cite{GatedConvolutionYu}}
\end{subfigure}%%
\begin{subfigure}[t]{0.2\textwidth}
\includegraphics[width=\textwidth]{images/comparisons/LBAM/places2/pluralistic/19.png}
\includegraphics[width=\textwidth]{images/comparisons/LBAM/places2/pluralistic/20.png}
\includegraphics[width=\textwidth]{images/comparisons/LBAM/places2/pluralistic/21.png}
\includegraphics[width=\textwidth]{images/comparisons/LBAM/places2/pluralistic/22.png}
\includegraphics[width=\textwidth]{images/comparisons/LBAM/places2/pluralistic/23.png}
\includegraphics[width=\textwidth]{images/comparisons/LBAM/places2/pluralistic/24.png}
\caption{PIC \cite{zheng2019pluralistic}}
\end{subfigure}%%
\begin{subfigure}[t]{0.2\textwidth}
\includegraphics[width=\textwidth]{images/comparisons/LBAM/places2/result/19.png}
\includegraphics[width=\textwidth]{images/comparisons/LBAM/places2/result/20.png}
\includegraphics[width=\textwidth]{images/comparisons/LBAM/places2/result/21.png}
\includegraphics[width=\textwidth]{images/comparisons/LBAM/places2/result/22.png}
\includegraphics[width=\textwidth]{images/comparisons/LBAM/places2/result/23.png}
\includegraphics[width=\textwidth]{images/comparisons/LBAM/places2/result/24.png}
\caption{Ours}
\end{subfigure}%%
\caption{\textbf{Places2 comparison to state-of-the-art models}
Examples selected by authors of \cite{BidirectionalAttentionXie} (images extracted from their supplementary material).
Results of \cite{GatedConvolutionYu,zheng2019pluralistic} generated by using their open-source code and models.
For comparisons to Patchmatch \cite{Barnes_2009}, Global \& Local Attention \cite{Iizuka_2017}, Contextual Attention \cite{ConextualAttention2018Yu}  and Partial Conv \cite{PconvLiu}, see \cite{BidirectionalAttentionXie}.
We recommend the reader to zoom-in on missing regions.}
\label{fig:LBAM_3}
\end{figure}
\begin{figure}[t]
\centering
\begin{subfigure}[t]{0.2\textwidth}
\includegraphics[width=\textwidth]{images/comparisons/LBAM/places2/masked_out/25.png}
\includegraphics[width=\textwidth]{images/comparisons/LBAM/places2/masked_out/26.png}
\includegraphics[width=\textwidth]{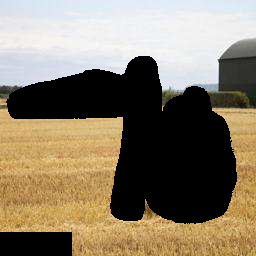}
\caption{Input}
\end{subfigure}%%
\begin{subfigure}[t]{0.2\textwidth}
\includegraphics[width=\textwidth]{images/comparisons/LBAM/places2/LBAM/25.png}
\includegraphics[width=\textwidth]{images/comparisons/LBAM/places2/LBAM/26.png}
\includegraphics[width=\textwidth]{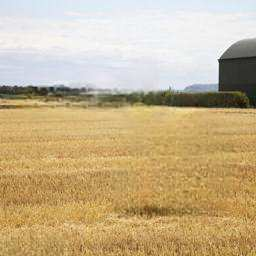}
\caption{LBAM \cite{BidirectionalAttentionXie}}
\end{subfigure}%%
\begin{subfigure}[t]{0.2\textwidth}
\includegraphics[width=\textwidth]{images/comparisons/LBAM/places2/gated_conv/25.png}
\includegraphics[width=\textwidth]{images/comparisons/LBAM/places2/gated_conv/26.png}
\includegraphics[width=\textwidth]{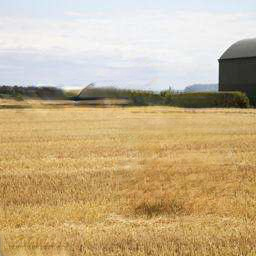}
\caption{GConv \cite{GatedConvolutionYu}}
\end{subfigure}%%
\begin{subfigure}[t]{0.2\textwidth}
\includegraphics[width=\textwidth]{images/comparisons/LBAM/places2/pluralistic/25.png}
\includegraphics[width=\textwidth]{images/comparisons/LBAM/places2/pluralistic/26.png}
\includegraphics[width=\textwidth]{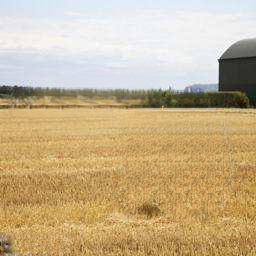}
\caption{PIC \cite{zheng2019pluralistic}}
\end{subfigure}%%
\begin{subfigure}[t]{0.2\textwidth}
\includegraphics[width=\textwidth]{images/comparisons/LBAM/places2/result/25.png}
\includegraphics[width=\textwidth]{images/comparisons/LBAM/places2/result/26.png}
\includegraphics[width=\textwidth]{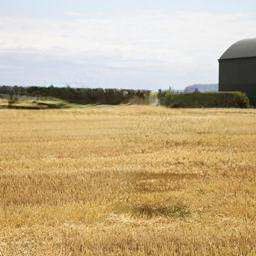}
\caption{Ours}
\end{subfigure}%%
\caption{\textbf{Places2 comparison to state-of-the-art models}
Examples selected by authors of \cite{BidirectionalAttentionXie} (images extracted from their supplementary material).
Results of \cite{GatedConvolutionYu,zheng2019pluralistic} generated by using their open-source code and models.
For comparisons to Patchmatch \cite{Barnes_2009}, Global \& Local Attention \cite{Iizuka_2017}, Contextual Attention \cite{ConextualAttention2018Yu}  and Partial Conv \cite{PconvLiu}, see \cite{BidirectionalAttentionXie}.
We recommend the reader to zoom-in on missing regions.}
\label{fig:LBAM_4}
\end{figure}
\begin{figure}[t]
\centering
\begin{subfigure}[t]{0.2\textwidth}
\includegraphics[width=\textwidth]{images/comparisons/FRRN/places2/masked_out/1.png}
\includegraphics[width=\textwidth]{images/comparisons/FRRN/places2/masked_out/2.png}
\includegraphics[width=\textwidth]{images/comparisons/FRRN/places2/masked_out/3.png}
\includegraphics[width=\textwidth]{images/comparisons/FRRN/places2/masked_out/5.png}
\includegraphics[width=\textwidth]{images/comparisons/FRRN/places2/masked_out/6.png}
\includegraphics[width=\textwidth]{images/comparisons/FRRN/places2/masked_out/7.png}
\caption{Input}
\end{subfigure}%%
\begin{subfigure}[t]{0.2\textwidth}
\includegraphics[width=\textwidth]{images/comparisons/FRRN/places2/gated_conv/1.png}
\includegraphics[width=\textwidth]{images/comparisons/FRRN/places2/gated_conv/2.png}
\includegraphics[width=\textwidth]{images/comparisons/FRRN/places2/gated_conv/3.png}
\includegraphics[width=\textwidth]{images/comparisons/FRRN/places2/gated_conv/5.png}
\includegraphics[width=\textwidth]{images/comparisons/FRRN/places2/gated_conv/6.png}
\includegraphics[width=\textwidth]{images/comparisons/FRRN/places2/gated_conv/7.png}
\caption{GConv \cite{GatedConvolutionYu}}
\end{subfigure}%%
\begin{subfigure}[t]{0.2\textwidth}
\includegraphics[width=\textwidth]{images/comparisons/FRRN/places2/pluralistic/1.png}
\includegraphics[width=\textwidth]{images/comparisons/FRRN/places2/pluralistic/2.png}
\includegraphics[width=\textwidth]{images/comparisons/FRRN/places2/pluralistic/3.png}
\includegraphics[width=\textwidth]{images/comparisons/FRRN/places2/pluralistic/5.png}
\includegraphics[width=\textwidth]{images/comparisons/FRRN/places2/pluralistic/6.png}
\includegraphics[width=\textwidth]{images/comparisons/FRRN/places2/pluralistic/7.png}
\caption{PIC \cite{zheng2019pluralistic}}
\end{subfigure}%%
\begin{subfigure}[t]{0.2\textwidth}
\includegraphics[width=\textwidth]{images/comparisons/FRRN/places2/FRRN/1.png}
\includegraphics[width=\textwidth]{images/comparisons/FRRN/places2/FRRN/2.png}
\includegraphics[width=\textwidth]{images/comparisons/FRRN/places2/FRRN/3.png}
\includegraphics[width=\textwidth]{images/comparisons/FRRN/places2/FRRN/5.png}
\includegraphics[width=\textwidth]{images/comparisons/FRRN/places2/FRRN/6.png}
\includegraphics[width=\textwidth]{images/comparisons/FRRN/places2/FRRN/7.png}
\caption{FRRN \cite{Guo_2019}}
\end{subfigure}%%
\begin{subfigure}[t]{0.2\textwidth}
\includegraphics[width=\textwidth]{images/comparisons/FRRN/places2/result/1.png}
\includegraphics[width=\textwidth]{images/comparisons/FRRN/places2/result/2.png}
\includegraphics[width=\textwidth]{images/comparisons/FRRN/places2/result/3.png}
\includegraphics[width=\textwidth]{images/comparisons/FRRN/places2/result/5.png}
\includegraphics[width=\textwidth]{images/comparisons/FRRN/places2/result/6.png}
\includegraphics[width=\textwidth]{images/comparisons/FRRN/places2/result/7.png}
\caption{Ours}
\end{subfigure}%%
\caption{\textbf{Places2 comparison to state-of-the-art models}
Examples selected by authors of \cite{Guo_2019} (images extracted from their paper).
Results of \cite{GatedConvolutionYu,zheng2019pluralistic} generated by using their open-source code and models.
Note that the original image size is $256 \times 256$.
We recommend the reader to zoom-in on missing regions.}
\label{fig:FRRN_0}
\end{figure}

\begin{figure}
\centering
\includegraphics[width=\textwidth]{images/deterministic/full.png}
\caption{
\textbf{Diverse Plausible Results:}
Images from the FDF validation dataset \cite{hukkelaas2019DeepPrivacy}.
Left column is the input image with the pose information marked in red.
Second column and onwards are different plausible generated results.
Each image is generated by randomly sampling a latent variable for the generator (except for the second column where the latent variable set to all 0's)}
\label{fig:deterministc_experiment_appendix}

\end{figure}
\begin{figure}
\centering
\includegraphics[width=\textwidth]{images/deterministic/random.png}
\caption{
\textbf{Diverse Plausible Results (Randomly Selected):}
Images from the FDF validation dataset \cite{hukkelaas2019DeepPrivacy}.
Left column is the input image with the pose information marked in red.
Second column and onwards are different plausible generated results.
Each image is generated by randomly sampling a latent variable for the generator (except for the second column where the latent variable set to all 0's).
All images are randomly selected.}
\label{fig:deterministc_experiment_appendix_random}

\end{figure}

\begin{figure}[!ht]
\centering
\begin{subfigure}[t]{0.25\textwidth}
\includegraphics[width=\textwidth]{images/comparisons/celebA-HQ/input/1068.png}
\includegraphics[width=\textwidth]{images/comparisons/celebA-HQ/input/643.png}
\includegraphics[width=\textwidth]{images/comparisons/celebA-HQ/input/1360.png}
\includegraphics[width=\textwidth]{images/comparisons/celebA-HQ/input/1878.png}
\caption{Input}
\end{subfigure}%%
\begin{subfigure}[t]{0.25\textwidth}
\includegraphics[width=\textwidth]{images/comparisons/celebA-HQ/gated_conv/1068.png}
\includegraphics[width=\textwidth]{images/comparisons/celebA-HQ/gated_conv/643.png}
\includegraphics[width=\textwidth]{images/comparisons/celebA-HQ/gated_conv/1360.png}
\includegraphics[width=\textwidth]{images/comparisons/celebA-HQ/gated_conv/1878.png}
\caption{GatedConv \cite{GatedConvolutionYu}}
\end{subfigure}%%
\begin{subfigure}[t]{0.25\textwidth}
\includegraphics[width=\textwidth]{images/comparisons/celebA-HQ/plurastic_inpainting/1068.png}
\includegraphics[width=\textwidth]{images/comparisons/celebA-HQ/plurastic_inpainting/643.png}
\includegraphics[width=\textwidth]{images/comparisons/celebA-HQ/plurastic_inpainting/1360.png}
\includegraphics[width=\textwidth]{images/comparisons/celebA-HQ/plurastic_inpainting/1878.png}
\caption{PIC \cite{zheng2019pluralistic}}
\end{subfigure}%%
\begin{subfigure}[t]{0.25\textwidth}
\includegraphics[width=\textwidth]{images/comparisons/celebA-HQ/result/1068.png}
\includegraphics[width=\textwidth]{images/comparisons/celebA-HQ/result/643.png}
\includegraphics[width=\textwidth]{images/comparisons/celebA-HQ/result/1360.png}
\includegraphics[width=\textwidth]{images/comparisons/celebA-HQ/result/1878.png}
\caption{Ours}
\end{subfigure}%%
\caption{
\textbf{CelebA-HQ (Center) comparisons to state-of-the-art image inpainting.}
Results are generated using open-source code and pre-trained models from the original authors.
All examples are randomly selected.}
\label{fig:celebA-HQ_randomly_0}
\end{figure}
\begin{figure}[!ht]
\centering
\begin{subfigure}[t]{0.25\textwidth}
\includegraphics[width=\textwidth]{images/comparisons/celebA-HQ/input/1086.png}
\includegraphics[width=\textwidth]{images/comparisons/celebA-HQ/input/1757.png}
\includegraphics[width=\textwidth]{images/comparisons/celebA-HQ/input/1289.png}
\includegraphics[width=\textwidth]{images/comparisons/celebA-HQ/input/1355.png}
\caption{Input}
\end{subfigure}%%
\begin{subfigure}[t]{0.25\textwidth}
\includegraphics[width=\textwidth]{images/comparisons/celebA-HQ/gated_conv/1086.png}
\includegraphics[width=\textwidth]{images/comparisons/celebA-HQ/gated_conv/1757.png}
\includegraphics[width=\textwidth]{images/comparisons/celebA-HQ/gated_conv/1289.png}
\includegraphics[width=\textwidth]{images/comparisons/celebA-HQ/gated_conv/1355.png}
\caption{GatedConv \cite{GatedConvolutionYu}}
\end{subfigure}%%
\begin{subfigure}[t]{0.25\textwidth}
\includegraphics[width=\textwidth]{images/comparisons/celebA-HQ/plurastic_inpainting/1086.png}
\includegraphics[width=\textwidth]{images/comparisons/celebA-HQ/plurastic_inpainting/1757.png}
\includegraphics[width=\textwidth]{images/comparisons/celebA-HQ/plurastic_inpainting/1289.png}
\includegraphics[width=\textwidth]{images/comparisons/celebA-HQ/plurastic_inpainting/1355.png}
\caption{PIC \cite{zheng2019pluralistic}}
\end{subfigure}%%
\begin{subfigure}[t]{0.25\textwidth}
\includegraphics[width=\textwidth]{images/comparisons/celebA-HQ/result/1086.png}
\includegraphics[width=\textwidth]{images/comparisons/celebA-HQ/result/1757.png}
\includegraphics[width=\textwidth]{images/comparisons/celebA-HQ/result/1289.png}
\includegraphics[width=\textwidth]{images/comparisons/celebA-HQ/result/1355.png}
\caption{Ours}
\end{subfigure}%%
\caption{
\textbf{CelebA-HQ (Center) comparisons to state-of-the-art image inpainting.}
Results are generated using open-source code and pre-trained models from the original authors.
All examples are randomly selected.}
\label{fig:celebA-HQ_randomly_1}
\end{figure}
\begin{figure}[!ht]
\centering
\begin{subfigure}[t]{0.25\textwidth}
\includegraphics[width=\textwidth]{images/comparisons/celebA-HQ_free_form/input/1397.png}
\includegraphics[width=\textwidth]{images/comparisons/celebA-HQ_free_form/input/1442.png}
\includegraphics[width=\textwidth]{images/comparisons/celebA-HQ_free_form/input/764.png}
\includegraphics[width=\textwidth]{images/comparisons/celebA-HQ_free_form/input/1674.png}
\caption{Input}
\end{subfigure}%%
\begin{subfigure}[t]{0.25\textwidth}
\includegraphics[width=\textwidth]{images/comparisons/celebA-HQ_free_form/gated_conv/1397.png}
\includegraphics[width=\textwidth]{images/comparisons/celebA-HQ_free_form/gated_conv/1442.png}
\includegraphics[width=\textwidth]{images/comparisons/celebA-HQ_free_form/gated_conv/764.png}
\includegraphics[width=\textwidth]{images/comparisons/celebA-HQ_free_form/gated_conv/1674.png}
\caption{GatedConv \cite{GatedConvolutionYu}}
\end{subfigure}%%
\begin{subfigure}[t]{0.25\textwidth}
\includegraphics[width=\textwidth]{images/comparisons/celebA-HQ_free_form/plurastic_inpainting/1397.png}
\includegraphics[width=\textwidth]{images/comparisons/celebA-HQ_free_form/plurastic_inpainting/1442.png}
\includegraphics[width=\textwidth]{images/comparisons/celebA-HQ_free_form/plurastic_inpainting/764.png}
\includegraphics[width=\textwidth]{images/comparisons/celebA-HQ_free_form/plurastic_inpainting/1674.png}
\caption{PIC \cite{zheng2019pluralistic}}
\end{subfigure}%%
\begin{subfigure}[t]{0.25\textwidth}
\includegraphics[width=\textwidth]{images/comparisons/celebA-HQ_free_form/result/1397.png}
\includegraphics[width=\textwidth]{images/comparisons/celebA-HQ_free_form/result/1442.png}
\includegraphics[width=\textwidth]{images/comparisons/celebA-HQ_free_form/result/764.png}
\includegraphics[width=\textwidth]{images/comparisons/celebA-HQ_free_form/result/1674.png}
\caption{Ours}
\end{subfigure}%%
\caption{
\textbf{CelebA-HQ (Free-Form) comparisons to state-of-the-art image inpainting.}
Results are generated using open-source code and pre-trained models from the original authors.
All examples are randomly selected.}
\label{fig:celebA-HQ_free_form_randomly_0}
\end{figure}
\begin{figure}[!ht]
\centering
\begin{subfigure}[t]{0.25\textwidth}
\includegraphics[width=\textwidth]{images/comparisons/celebA-HQ_free_form/input/2023.png}
\includegraphics[width=\textwidth]{images/comparisons/celebA-HQ_free_form/input/646.png}
\includegraphics[width=\textwidth]{images/comparisons/celebA-HQ_free_form/input/558.png}
\includegraphics[width=\textwidth]{images/comparisons/celebA-HQ_free_form/input/2371.png}
\caption{Input}
\end{subfigure}%%
\begin{subfigure}[t]{0.25\textwidth}
\includegraphics[width=\textwidth]{images/comparisons/celebA-HQ_free_form/gated_conv/2023.png}
\includegraphics[width=\textwidth]{images/comparisons/celebA-HQ_free_form/gated_conv/646.png}
\includegraphics[width=\textwidth]{images/comparisons/celebA-HQ_free_form/gated_conv/558.png}
\includegraphics[width=\textwidth]{images/comparisons/celebA-HQ_free_form/gated_conv/2371.png}
\caption{GatedConv \cite{GatedConvolutionYu}}
\end{subfigure}%%
\begin{subfigure}[t]{0.25\textwidth}
\includegraphics[width=\textwidth]{images/comparisons/celebA-HQ_free_form/plurastic_inpainting/2023.png}
\includegraphics[width=\textwidth]{images/comparisons/celebA-HQ_free_form/plurastic_inpainting/646.png}
\includegraphics[width=\textwidth]{images/comparisons/celebA-HQ_free_form/plurastic_inpainting/558.png}
\includegraphics[width=\textwidth]{images/comparisons/celebA-HQ_free_form/plurastic_inpainting/2371.png}
\caption{PIC \cite{zheng2019pluralistic}}
\end{subfigure}%%
\begin{subfigure}[t]{0.25\textwidth}
\includegraphics[width=\textwidth]{images/comparisons/celebA-HQ_free_form/result/2023.png}
\includegraphics[width=\textwidth]{images/comparisons/celebA-HQ_free_form/result/646.png}
\includegraphics[width=\textwidth]{images/comparisons/celebA-HQ_free_form/result/558.png}
\includegraphics[width=\textwidth]{images/comparisons/celebA-HQ_free_form/result/2371.png}
\caption{Ours}
\end{subfigure}%%
\caption{
\textbf{CelebA-HQ (Free-Form) comparisons to state-of-the-art image inpainting.}
Results are generated using open-source code and pre-trained models from the original authors.
All examples are randomly selected.}
\label{fig:celebA-HQ_free_form_randomly_1}
\end{figure}
\begin{figure}[!ht]
\centering
\begin{subfigure}[t]{0.25\textwidth}
\includegraphics[width=\textwidth]{images/comparisons/places2/input/642.png}
\includegraphics[width=\textwidth]{images/comparisons/places2/input/12279.png}
\includegraphics[width=\textwidth]{images/comparisons/places2/input/7494.png}
\includegraphics[width=\textwidth]{images/comparisons/places2/input/28251.png}
\caption{Input}
\end{subfigure}%%
\begin{subfigure}[t]{0.25\textwidth}
\includegraphics[width=\textwidth]{images/comparisons/places2/gated_conv/642.png}
\includegraphics[width=\textwidth]{images/comparisons/places2/gated_conv/12279.png}
\includegraphics[width=\textwidth]{images/comparisons/places2/gated_conv/7494.png}
\includegraphics[width=\textwidth]{images/comparisons/places2/gated_conv/28251.png}
\caption{GatedConv \cite{GatedConvolutionYu}}
\end{subfigure}%%
\begin{subfigure}[t]{0.25\textwidth}
\includegraphics[width=\textwidth]{images/comparisons/places2/plurastic_inpainting/642.png}
\includegraphics[width=\textwidth]{images/comparisons/places2/plurastic_inpainting/12279.png}
\includegraphics[width=\textwidth]{images/comparisons/places2/plurastic_inpainting/7494.png}
\includegraphics[width=\textwidth]{images/comparisons/places2/plurastic_inpainting/28251.png}
\caption{PIC \cite{zheng2019pluralistic}}
\end{subfigure}%%
\begin{subfigure}[t]{0.25\textwidth}
\includegraphics[width=\textwidth]{images/comparisons/places2/result/642.png}
\includegraphics[width=\textwidth]{images/comparisons/places2/result/12279.png}
\includegraphics[width=\textwidth]{images/comparisons/places2/result/7494.png}
\includegraphics[width=\textwidth]{images/comparisons/places2/result/28251.png}
\caption{Ours}
\end{subfigure}%%
\caption{
\textbf{Places2 (Center) comparisons to state-of-the-art image inpainting.}
Results are generated using open-source code and pre-trained models from the original authors.
All examples are randomly selected.}
\label{fig:places2_randomly_0}
\end{figure}
\begin{figure}[!ht]
\centering
\begin{subfigure}[t]{0.25\textwidth}
\includegraphics[width=\textwidth]{images/comparisons/places2/input/8566.png}
\includegraphics[width=\textwidth]{images/comparisons/places2/input/15053.png}
\includegraphics[width=\textwidth]{images/comparisons/places2/input/15749.png}
\includegraphics[width=\textwidth]{images/comparisons/places2/input/1410.png}
\caption{Input}
\end{subfigure}%%
\begin{subfigure}[t]{0.25\textwidth}
\includegraphics[width=\textwidth]{images/comparisons/places2/gated_conv/8566.png}
\includegraphics[width=\textwidth]{images/comparisons/places2/gated_conv/15053.png}
\includegraphics[width=\textwidth]{images/comparisons/places2/gated_conv/15749.png}
\includegraphics[width=\textwidth]{images/comparisons/places2/gated_conv/1410.png}
\caption{GatedConv \cite{GatedConvolutionYu}}
\end{subfigure}%%
\begin{subfigure}[t]{0.25\textwidth}
\includegraphics[width=\textwidth]{images/comparisons/places2/plurastic_inpainting/8566.png}
\includegraphics[width=\textwidth]{images/comparisons/places2/plurastic_inpainting/15053.png}
\includegraphics[width=\textwidth]{images/comparisons/places2/plurastic_inpainting/15749.png}
\includegraphics[width=\textwidth]{images/comparisons/places2/plurastic_inpainting/1410.png}
\caption{PIC \cite{zheng2019pluralistic}}
\end{subfigure}%%
\begin{subfigure}[t]{0.25\textwidth}
\includegraphics[width=\textwidth]{images/comparisons/places2/result/8566.png}
\includegraphics[width=\textwidth]{images/comparisons/places2/result/15053.png}
\includegraphics[width=\textwidth]{images/comparisons/places2/result/15749.png}
\includegraphics[width=\textwidth]{images/comparisons/places2/result/1410.png}
\caption{Ours}
\end{subfigure}%%
\caption{
\textbf{Places2 (Center) comparisons to state-of-the-art image inpainting.}
Results are generated using open-source code and pre-trained models from the original authors.
All examples are randomly selected.}
\label{fig:places2_randomly_1}
\end{figure}
\begin{figure}[!ht]
\centering
\begin{subfigure}[t]{0.25\textwidth}
\includegraphics[width=\textwidth]{images/comparisons/places2_free_form/input/14923.png}
\includegraphics[width=\textwidth]{images/comparisons/places2_free_form/input/28540.png}
\includegraphics[width=\textwidth]{images/comparisons/places2_free_form/input/31349.png}
\includegraphics[width=\textwidth]{images/comparisons/places2_free_form/input/34526.png}
\caption{Input}
\end{subfigure}%%
\begin{subfigure}[t]{0.25\textwidth}
\includegraphics[width=\textwidth]{images/comparisons/places2_free_form/gated_conv/14923.png}
\includegraphics[width=\textwidth]{images/comparisons/places2_free_form/gated_conv/28540.png}
\includegraphics[width=\textwidth]{images/comparisons/places2_free_form/gated_conv/31349.png}
\includegraphics[width=\textwidth]{images/comparisons/places2_free_form/gated_conv/34526.png}
\caption{GatedConv \cite{GatedConvolutionYu}}
\end{subfigure}%%
\begin{subfigure}[t]{0.25\textwidth}
\includegraphics[width=\textwidth]{images/comparisons/places2_free_form/plurastic_inpainting/14923.png}
\includegraphics[width=\textwidth]{images/comparisons/places2_free_form/plurastic_inpainting/28540.png}
\includegraphics[width=\textwidth]{images/comparisons/places2_free_form/plurastic_inpainting/31349.png}
\includegraphics[width=\textwidth]{images/comparisons/places2_free_form/plurastic_inpainting/34526.png}
\caption{PIC \cite{zheng2019pluralistic}}
\end{subfigure}%%
\begin{subfigure}[t]{0.25\textwidth}
\includegraphics[width=\textwidth]{images/comparisons/places2_free_form/result/14923.png}
\includegraphics[width=\textwidth]{images/comparisons/places2_free_form/result/28540.png}
\includegraphics[width=\textwidth]{images/comparisons/places2_free_form/result/31349.png}
\includegraphics[width=\textwidth]{images/comparisons/places2_free_form/result/34526.png}
\caption{Ours}
\end{subfigure}%%
\caption{
\textbf{Places2 (Free-Form) comparisons to state-of-the-art image inpainting.}
Results are generated using open-source code and pre-trained models from the original authors.
All examples are randomly selected.}
\label{fig:places2_free_form_randomly_0}
\end{figure}
\begin{figure}[!ht]
\centering
\begin{subfigure}[t]{0.25\textwidth}
\includegraphics[width=\textwidth]{images/comparisons/places2_free_form/input/29145.png}
\includegraphics[width=\textwidth]{images/comparisons/places2_free_form/input/712.png}
\includegraphics[width=\textwidth]{images/comparisons/places2_free_form/input/20702.png}
\includegraphics[width=\textwidth]{images/comparisons/places2_free_form/input/23534.png}
\caption{Input}
\end{subfigure}%%
\begin{subfigure}[t]{0.25\textwidth}
\includegraphics[width=\textwidth]{images/comparisons/places2_free_form/gated_conv/29145.png}
\includegraphics[width=\textwidth]{images/comparisons/places2_free_form/gated_conv/712.png}
\includegraphics[width=\textwidth]{images/comparisons/places2_free_form/gated_conv/20702.png}
\includegraphics[width=\textwidth]{images/comparisons/places2_free_form/gated_conv/23534.png}
\caption{GatedConv \cite{GatedConvolutionYu}}
\end{subfigure}%%
\begin{subfigure}[t]{0.25\textwidth}
\includegraphics[width=\textwidth]{images/comparisons/places2_free_form/plurastic_inpainting/29145.png}
\includegraphics[width=\textwidth]{images/comparisons/places2_free_form/plurastic_inpainting/712.png}
\includegraphics[width=\textwidth]{images/comparisons/places2_free_form/plurastic_inpainting/20702.png}
\includegraphics[width=\textwidth]{images/comparisons/places2_free_form/plurastic_inpainting/23534.png}
\caption{PIC \cite{zheng2019pluralistic}}
\end{subfigure}%%
\begin{subfigure}[t]{0.25\textwidth}
\includegraphics[width=\textwidth]{images/comparisons/places2_free_form/result/29145.png}
\includegraphics[width=\textwidth]{images/comparisons/places2_free_form/result/712.png}
\includegraphics[width=\textwidth]{images/comparisons/places2_free_form/result/20702.png}
\includegraphics[width=\textwidth]{images/comparisons/places2_free_form/result/23534.png}
\caption{Ours}
\end{subfigure}%%
\caption{
\textbf{Places2 (Free-Form) comparisons to state-of-the-art image inpainting.}
Results are generated using open-source code and pre-trained models from the original authors.
All examples are randomly selected.}
\label{fig:places2_free_form_randomly_1}
\end{figure}
